# Supplementary material for: Belief Coevolution in a Social Network of Generalist and Specialist Large Language Models: A Controlled Study
Source: arXiv:2607.27512 source file (2026-10-18)
Supplement: Supplementary file 1 [file fingerprint_data.tex]

\fpbucket{1}{Focus}
  \fpcat{1}{bel}{Belief / opinion dynamics}
  \fpcat{1}{beh}{Behavior (selected)}
\fpbucket{2}{Personas}
  \fpcat{2}{id}{Identity personas}
  \fpcat{2}{ftp}{Personas via fine-tuning}
  \fpcat{2}{fun}{Functional roles only}
  \fpcat{2}{none}{No personas}
  \fpcat{2}{unc}{Unclear}
\fpbucket{3}{Specialists}
  \fpcat{3}{dom}{Domain-specialist LLMs}
  \fpcat{3}{none}{No domain specialists}
\fpbucket{5}{Population}
  \fpcat{5}{het}{Heterogeneous LLMs}
  \fpcat{5}{both}{Both (compared)}
  \fpcat{5}{hom}{Homogeneous}
  \fpcat{5}{unc}{Unclear}
\fpbucket{6}{Communication}
  \fpcat{6}{sum}{Discrete-belief summary}
  \fpcat{6}{bcast}{Answer broadcast}
  \fpcat{6}{debate}{Structured debate}
  \fpcat{6}{dialog}{Free-form dialogue}
  \fpcat{6}{chat}{Group chat / shared memory}
  \fpcat{6}{posts}{Social-media posts}
  \fpcat{6}{game}{Game actions}
  \fpcat{6}{obs}{Observational platform}
\fpbucket{7}{Structure}
  \fpcat{7}{net}{Explicit network}
  \fpcat{7}{full}{Fully connected group}
  \fpcat{7}{judge}{Debaters + judge}
  \fpcat{7}{dyad}{Dyad}
  \fpcat{7}{pairs}{Random pairs}
  \fpcat{7}{env}{Environment / sandbox}
  \fpcat{7}{emerg}{Emergent platform}

\fpours{bel}{id}{dom}{yes}{both}{sum}{net}
\fpoursrow

\fppaper{\fpcite{chen2025multiagentconsensusseekinglarge}}{n}{bel}{id}{none}{no}{hom}{bcast}{net}   % Chen '23
\fppaper{\fpcite{cho2025herdbehaviorinvestigatingpeer}}{n}{bel}{id}{none}{no}{hom}{sum}{full}   % Cho '25
\fppaper{\fpcite{Gu2026LanguageGroundedCO}}{n}{bel}{id}{none}{no}{hom}{posts}{net}   % Gu '26
\fppaper{\fpcite{jiang2026agentbasedmodelingequilibriumecho}}{n}{bel}{id}{none}{no}{hom}{posts}{net}   % Jiang '26
\fppaper{\fpcite{mehdizadeh2025aiagentsuccumbspeerpressure}}{n}{bel}{none}{none}{no}{hom}{sum}{net}   % Mehdizadeh '25
\fppaper{\fpcite{yazici2026opinion}}{n}{bel}{id}{none}{no}{unc}{bcast}{net}   % Yazici '26
\fppaper{\fpcite{ye2026stop}}{n}{bel}{id}{none}{partial}{hom}{posts}{net}   % Ye '26
\fppaper{\fpcite{baltaji-etal-2024-conformity}}{n}{bel}{id}{none}{no}{hom}{chat}{full}   % Baltaji '24
\fppaper{\fpcite{bilgin_effect_2025}}{n}{bel}{id}{none}{no}{hom}{debate}{dyad}   % Bilgin '25
\fppaper{\fpcite{cau2026collectiveopiniondynamicsstructured}}{n}{bel}{none}{none}{no}{hom}{debate}{net}   % Cau '26
\fppaper{\fpcite{chuang-etal-2024-simulating}}{n}{bel}{id}{none}{no}{hom}{dialog}{pairs}   % Chuang '24
\fppaper{\fpcite{demarzo_aiagents}}{n}{bel}{none}{none}{no}{hom}{sum}{full}   % De Marzo '24
\fppaper{\fpcite{demarzo2026conformitygeneratescollectivemisalignment}}{n}{bel}{none}{none}{no}{hom}{sum}{full}   % De Marzo '26
\fppaper{\fpcite{gao_s3_2023}}{n}{bel}{ftp}{none}{no}{hom}{posts}{net}   % Gao '23
\fppaper{\fpcite{he2026opiniondynamicsmutualinfluence}}{n}{bel}{none}{none}{no}{both}{posts}{full}   % He '26
\fppaper{\fpcite{ko2026attractor}}{n}{bel}{none}{none}{partial}{both}{debate}{dyad}   % Ko '26
\fppaper{\fpcite{liu-etal-2025-synthetic}}{n}{bel}{id}{none}{no}{hom}{debate}{dyad}   % Liu '25
\fppaper{\fpcite{laustsen2026peerinfluenceheterogeneousai}}{n}{bel}{none}{none}{partial}{both}{bcast}{dyad}   % Nøhr Laustsen '26
\fppaper{\fpcite{piao2025agentsociety}}{n}{bel}{id}{none}{no}{hom}{posts}{env}   % Piao '25
\fppaper{\fpcite{probine2026characterizingopinionevolutionnetworked}}{n}{bel}{none}{none}{no}{hom}{posts}{net}   % Probine '26
\fppaper{\fpcite{zhang2025socioverse}}{n}{bel}{id}{none}{no}{hom}{posts}{env}   % Zhang '25
\fppaper{\fpcite{breum_persuasive_2024}}{n}{bel}{fun}{none}{no}{hom}{dialog}{dyad}   % Breum '24
\fppaper{\fpcite{brockers_disentangling_2026}}{n}{bel}{ftp}{none}{partial}{hom}{dialog}{dyad}   % Brockers '25
\fppaper{\fpcite{cau_selective_2025}}{n}{bel}{none}{none}{no}{hom}{debate}{pairs}   % Cau '25
\fppaper{\fpcite{chuang2025debate}}{n}{bel}{ftp}{none}{no}{hom}{chat}{full}   % Chuang '25
\fppaper{\fpcite{nguyen_two_2025}}{n}{bel}{none}{none}{no}{hom}{debate}{dyad}   % Nguyen '25
\fppaper{\fpcite{payandeh-etal-2024-susceptible}}{n}{bel}{fun}{none}{no}{unc}{debate}{judge}   % Payandeh '24
\fppaper{\fpcite{taubenfeld-etal-2024-systematic}}{n}{bel}{ftp}{none}{no}{hom}{debate}{full}   % Taubenfeld '24
\fppaper{\fpcite{wang-etal-2023-chatgpt-defend}}{n}{bel}{none}{none}{no}{hom}{dialog}{dyad}   % Wang '23
\fpblock
\fppaper{\fpcite{bhandari-etal-2025-llm,robotics13050068}}{n}{beh}{id}{none}{no}{het}{debate}{dyad}   % Bhandari '25
\fppaper{\fpcite{estornell_multi-llm_2024}}{n}{beh}{none}{none}{no}{both}{bcast}{full}   % Estornell '24
\fppaper{\fpcite{li-etal-2024-simulating}}{n}{beh}{id}{none}{no}{hom}{bcast}{full}   % Li '24
\fppaper{\fpcite{chen-etal-2024-reconcile}}{n}{beh}{none}{dom}{partial}{het}{bcast}{full}   % ReConcile '24
\fppaper{\fpcite{ashery2025emergent}}{n}{beh}{none}{none}{no}{hom}{game}{pairs}   % Ashery '25
\fppaper{\fpcite{flint_groupsize}}{n}{beh}{none}{none}{no}{hom}{game}{pairs}   % Flint '26 (group size)
\fppaper{\fpcite{flint2026indirecttippingsocialattack}}{n}{beh}{none}{none}{no}{hom}{game}{pairs}   % Flint '26 (tipping)
\fppaper{\fpcite{li2026does}}{n}{beh}{unc}{none}{no}{het}{obs}{emerg}   % Li '26
\fppaper{\fpcite{parfenova2025tracing}}{n}{beh}{none}{none}{no}{het}{chat}{full}   % Parfenova '25
\fppaper{\fpcite{xiong-etal-2023-examining}}{n}{beh}{none}{none}{no}{het}{debate}{judge}   % Xiong '23
