# Supplementary material for: Belief Coevolution in a Social Network of Generalist and Specialist Large Language Models: A Controlled Study
Source: arXiv:2607.27512 source file (2026-10-18)
Supplement: Supplementary file 2 [file fingerprint_macros.tex]

======================================================================
\makeatletter
\definecolor{fpaccent}{HTML}{B4B341}   % highlight (dots, stars)
\definecolor{fpshade}{HTML}{F4F4E3}    % shaded CoevolveSim columns
\definecolor{fptext}{HTML}{6B6A1F}     % accent-coloured text
\definecolor{fpdot}{HTML}{5F5E5A}      % non-matching dots
\definecolor{fprule}{HTML}{B4B2A9}
\pgfdeclarelayer{fpbg}\pgfsetlayers{fpbg,main}


\providecommand{\fpcite}[1]{\ifdefined\citet\citet{#1}\else\cite{#1}\fi}


\providecommand{\fpskip}{4}

% ---- layout parameters (cm) ----
\def\fpcolw{0.42}   % width of one category column
\def\fpgapw{0.45}   % extra gap between buckets
\def\fprowh{0.36}   % row height
\def\fpblockgap{0.25}
\def\fpnbuckets{7}

\newcounter{fpcol}\newcounter{fprow}\newcounter{fpmatch}\newcounter{fpbk}\newcounter{fpshown}
\newcommand{\fpden}{\the\numexpr7-\ifnum\fpskip>0 1\else 0\fi\relax}
\newcommand{\fpright}{\the\value{fpcol}*\fpcolw+(\the\value{fpshown}-1)*\fpgapw}
\def\fpy{0}

\newcommand{\fpbucket}[2]{%
  \setcounter{fpbk}{#1}\csgdef{fpbname@#1}{#2}%
  \ifnumequal{#1}{\fpskip}{}{\stepcounter{fpshown}}%
  \csxdef{fpbidx@#1}{\the\value{fpshown}}%
  \csxdef{fpbfirst@#1}{\the\numexpr\value{fpcol}+1\relax}}
\newcommand{\fpcat}[3]{\ifnumequal{#1}{\fpskip}{}{%
  \stepcounter{fpcol}%
  \pgfmathsetmacro\fptmp{\the\value{fpcol}*\fpcolw+(\csuse{fpbidx@#1}-1)*\fpgapw}%
  \csxdef{fpx@#1@#2}{\fptmp}\csgdef{fplab@#1@#2}{#3}%
  \csxdef{fpblast@#1}{\the\value{fpcol}}%
  \node[rotate=60,anchor=south west,inner sep=1pt,font=\scriptsize] at (\fptmp,0.12) {#3};}}
\newcommand{\fpours}[7]{%
  \gdef\fpo@i{#1}\gdef\fpo@ii{#2}\gdef\fpo@iii{#3}\gdef\fpo@iv{#4}%
  \gdef\fpo@v{#5}\gdef\fpo@vi{#6}\gdef\fpo@vii{#7}}
\newcommand{\fp@dot}[3]{\ifnumequal{#2}{\fpskip}{}{\fp@@dot{#1}{#2}{#3}}}
\newcommand{\fp@@dot}[3]{% bucket roman, bucket number, key
  \ifcsdef{fpx@#2@#3}{%
    \ifcsstring{fpo@#1}{#3}%
      {\stepcounter{fpmatch}\fill[fpaccent] (\csuse{fpx@#2@#3},\fpy) circle (0.075);}%
      {\fill[fpdot] (\csuse{fpx@#2@#3},\fpy) circle (0.075);}}%
    {\PackageWarning{fingerprint}{Unknown key '#3' in bucket #2 -- add an \string\fpcat}}}
\newcommand{\fppaper}[9]{%
  \stepcounter{fprow}\setcounter{fpmatch}{0}%
  \pgfmathsetmacro\fpy{\fpy-\fprowh}\xdef\fpy{\fpy}%
  \ifstrequal{#2}{i}%
    {\node[anchor=east,font=\scriptsize\itshape,text=fpdot] at (0,\fpy) {#1};}%
    {\node[anchor=east,font=\scriptsize] at (0,\fpy) {#1};}%
  \fp@dot{i}{1}{#3}\fp@dot{ii}{2}{#4}\fp@dot{iii}{3}{#5}\fp@dot{iv}{4}{#6}%
  \fp@dot{v}{5}{#7}\fp@dot{vi}{6}{#8}\fp@dot{vii}{7}{#9}%
  \pgfmathsetmacro\fpxr{\fpright+0.45}%
  \node[anchor=west,font=\scriptsize,text=fpdot] at (\fpxr,\fpy) {\arabic{fpmatch}/\fpden};}
\newcommand{\fp@star}[2]{\ifnumequal{#2}{\fpskip}{}{\node[text=fpaccent,inner sep=0pt,font=\small] at (\csuse{fpx@#2@\csuse{fpo@#1}},\fpy) {$\star$};}}
\newcommand{\fpoursrow}{%
  \pgfmathsetmacro\fpy{\fpy-\fprowh}\xdef\fpy{\fpy}%
  \node[anchor=east,font=\scriptsize\bfseries,text=fptext] at (0,\fpy) {CoevolveSim};
  \fp@star{i}{1}\fp@star{ii}{2}\fp@star{iii}{3}\fp@star{iv}{4}\fp@star{v}{5}\fp@star{vi}{6}\fp@star{vii}{7}%
  \pgfmathsetmacro\fpxr{\fpright+0.45}%
  \node[anchor=west,font=\scriptsize\bfseries,text=fptext] at (\fpxr,\fpy) {\fpden/\fpden};
  \pgfmathsetmacro\fpy{\fpy-0.08}\xdef\fpy{\fpy}%
  \draw[fprule,line width=0.3pt] (-3.2,\fpy) -- (\fpxr+0.7,\fpy);}
\newcommand{\fpblock}{%
  \pgfmathsetmacro\fpy{\fpy-\fpblockgap}\xdef\fpy{\fpy}%
  \pgfmathsetmacro\fpxr{\fpright+1.15}%
  \draw[fprule,line width=0.3pt] (-3.2,\fpy+0.05) -- (\fpxr,\fpy+0.05);}
\newcommand{\fpcaption}[1]{%
  \pgfmathsetmacro\fpxr{\fpright+1.15}%
  \node[anchor=north west,font=\scriptsize,text=fpdot,text width=(\fpxr+3.2)*1cm,align=left,inner sep=0pt] at (-3.2,\fpy-0.35) {#1};}
\newcommand{\fp@shade}[2]{\ifnumequal{#2}{\fpskip}{}{\fp@@shade{#1}{#2}}}
\newcommand{\fp@@shade}[2]{\pgfmathsetmacro\fpsx{\csuse{fpx@#2@\csuse{fpo@#1}}}%
  \begin{pgfonlayer}{fpbg}\fill[fpshade] (\fpsx-0.17,0.05) rectangle (\fpsx+0.17,\fpy-0.2);\end{pgfonlayer}}
\newcommand{\fp@head}[1]{\ifnumequal{#1}{\fpskip}{}{\fp@@head{#1}}}
\newcommand{\fp@@head}[1]{%
  \pgfmathsetmacro\fpa{\csuse{fpbfirst@#1}*\fpcolw+(\csuse{fpbidx@#1}-1)*\fpgapw-0.12}%
  \pgfmathsetmacro\fpb{\csuse{fpblast@#1}*\fpcolw+(\csuse{fpbidx@#1}-1)*\fpgapw+0.12}%
  \draw[fprule,line width=0.4pt] (\fpa,0.05) -- (\fpb,0.05);
  \draw[fprule,line width=0.4pt] (\fpa,3.55) -- (\fpb,3.55);
  \node[font=\scriptsize\bfseries,anchor=south,align=center,inner sep=1pt] at ({(\fpa+\fpb)/2},3.6) {\csuse{fpbname@#1}};}
\newcommand{\fpfinish}{%
  \fp@shade{i}{1}\fp@shade{ii}{2}\fp@shade{iii}{3}\fp@shade{iv}{4}%
  \fp@shade{v}{5}\fp@shade{vi}{6}\fp@shade{vii}{7}%
  \foreach \b in {1,...,7}{\fp@head{\b}}}
\makeatother
